# Supplementary material for: SAIL-Embedding Technical Report: Omni-modal Embedding Foundation Model
Source: arXiv:2510.12709 source file (2025-11-02)
Supplement: Supplementary file 1 [file appendix.tex]

% \section{Appendix}
% \subsection{Secondary Level Headings}
% \subsubsection{Three Level Headings}
% \vspace{0.3pt}\noindent\textbf{Fourth Level Headings}\hspace{1ex}
% This is used to test the format of the content.
